# Supplementary material for: MTVNet: Mapping using Transformers for Volumes -- Network for Super-Resolution with Long-Range Interactions
Source: arXiv:2412.03379 source file (2024-12-09)
Supplement: Supplementary file 1 [file 12_appendix.tex]

\section{Appendix Section}
\label{sec:appendix_section}
Supplementary material goes here.

\begin{figure}[t]
   \centering
   %\fbox{\rule{0pt}{2in} \rule{0.9\linewidth}{0pt}}
   \includegraphics[width=0.55\linewidth]{figs/svhat_layer_V2.pdf}
   \caption{Overview of proposed SVHAT layer that captures global and local token dependencies using separate attention branches for CATs (\textcolor{blue}{blue}) and ITEs (\textcolor{red}{red}). The first branch follows the attention procedure from FasterViT \cite{Hatamizadeh_FasterViT}, whereas the second follows the approach from SwinV2 \cite{Liu_SwinV2}. We use CSM modules to merge tokens from preceding levels before computing attention in each branch.}
   \label{fig:svhat_layer}
\end{figure}
