# Supplementary material for: MTVNet: Mapping using Transformers for Volumes -- Network for Super-Resolution with Long-Range Interactions
Source: arXiv:2412.03379 source file (2024-12-09)
Supplement: Supplementary file 2 [file A1_suppl_2.tex]

\clearpage
\setcounter{page}{1}
\maketitlesupplementary

\section{Details of SVHAT layer}

\begin{figure}[h]
   \centering
   %\fbox{\rule{0pt}{2in} \rule{0.9\linewidth}{0pt}}
   \includegraphics[width=0.8\linewidth]{figs/svhat_overview_2_2.pdf}
   \caption{Overview of proposed SVHAT layer that captures global and local token dependencies using separate attention branches for CATs (\textcolor{red}{red}) and ITEs (\textcolor{blue}{blue}). The first branch follows the attention procedure from FasterViT \cite{Hatamizadeh_FasterViT}, whereas the second follows the approach from SwinV2 \cite{Liu_SwinV2}. We use CSM modules to merge tokens from preceding levels before computing attention in each branch.}
   \label{fig:svhat_layer}
\end{figure}

\section{Training details}

\subsection{Datasets}

\textbf{Human Connectome Project (HCP) 1200}\\ The HCP 1200 Subjects Data Release \cite{Van_HCP_1200_dataset} includes structural MRI scans from 1113 healthy subjects acquired using a 3T scanning platform. We use the T1-weighted images, featuring an isotropic resolution of 0.7 mm and a matrix size of $320\times320\times256$. Following \cite{Chen_mDCSRN_C, Forigua_SuperFormer}, the dataset is split into 780 subjects for training, and 111 each for validation, evaluation, and testing. Performance evaluation is conducted solely on the test set.

\textbf{Information eXtraction from Images (IXI)}\\ The IXI dataset contains multi-modality MRI data (PD-, T1-, and T2-weighted) from 600 healthy subjects scanned with one 3T and two 1.5T scanning platforms. We use 581 T1-weighted scans, of which 507 have a resolution of $0.9375\times0.9375\times1.2$ mm and a matrix size of $256\times256\times150$, while the remaining 74 have a similar resolution but a matrix size of $256\times256\times146$. The dataset is split into 500 subjects for training, 6 for validation, and 75 for testing, with evaluation performed on the test set.

\textbf{Brain Tumor Segmentation Challenge (BraTS) 2023}\\ For BraTS 2023, we use 1470 T1-weighted skull-stripped MRI scans of glioma patients, standardized to an isotropic resolution of 1 mm and a matrix size of $240\times240\times155$. The provided dataset split allocates 1251 subjects for training and 219 for validation, with evaluation performed on the validation set.

\textbf{Kirby 21}\\ The Kirby 21 dataset includes multi-modality MRI scans from healthy individuals with no history of neurological conditions. We use the 42 T2-weighted images, which have a resolution of $1\times0.9375\times0.9375$ mm and a matrix size of $180\times256\times256$. The data is split into 37 images for training (KKI-06 to KKI-42) and 5 for testing (KKI-01 to KKI-05).

\textbf{Femur Archaeological CT Superresolution (FACTS)}\\ The FACTS dataset comprises 12 archaeological proximal femurs scanned with clinical-CT and micro-CT platforms \cite{Bardenfleth_FACTS}. Clinical-CT scans have a resolution of $0.21\times0.21\times0.4$ mm, while micro-CT scans have a resolution of $58\times58\times58$ $\mu$m. Clinical-CT volumes are registered and linearly interpolated to match the micro-CT matrix size. The dataset is split into 10 images for training and 2 (f\_002 and f\_138) for testing.

\begin{figure}[t]
    \centering
        \begin{subfigure}{\linewidth}
        \includegraphics[width=1.0\linewidth]{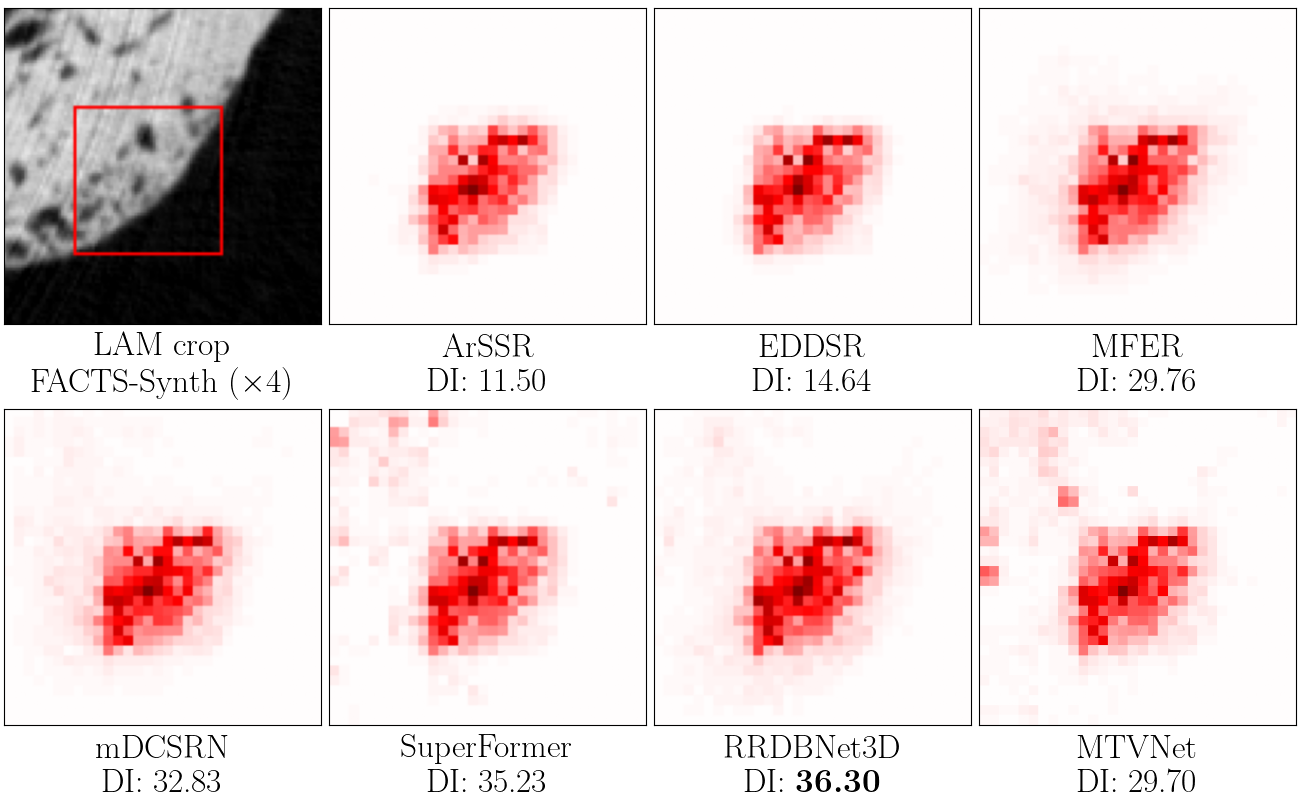}
        %\caption{LAM comparison of SR models from FACTS-Synth at $4 \times$ upscaling.}
        %\label{fig:LAM_visualisation}
        \end{subfigure}
        \begin{subfigure}{\linewidth}
        \includegraphics[width=1.0\linewidth]{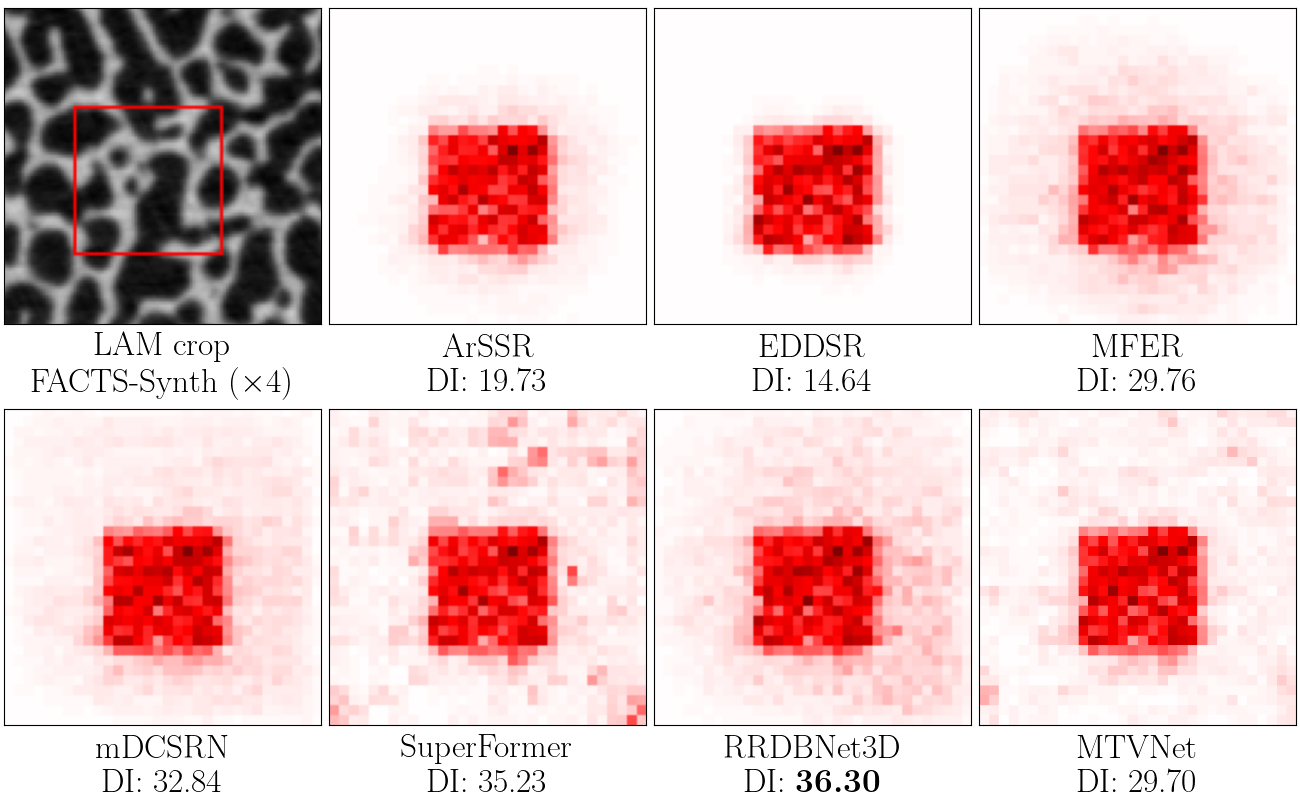}
        %\caption{LAM comparison of SR models from FACTS-Synth at $4 \times$ upscaling.}
        %\label{fig:LAM_visualisation}
        \end{subfigure}
        \begin{subfigure}{\linewidth}
        \includegraphics[width=1.0\linewidth]{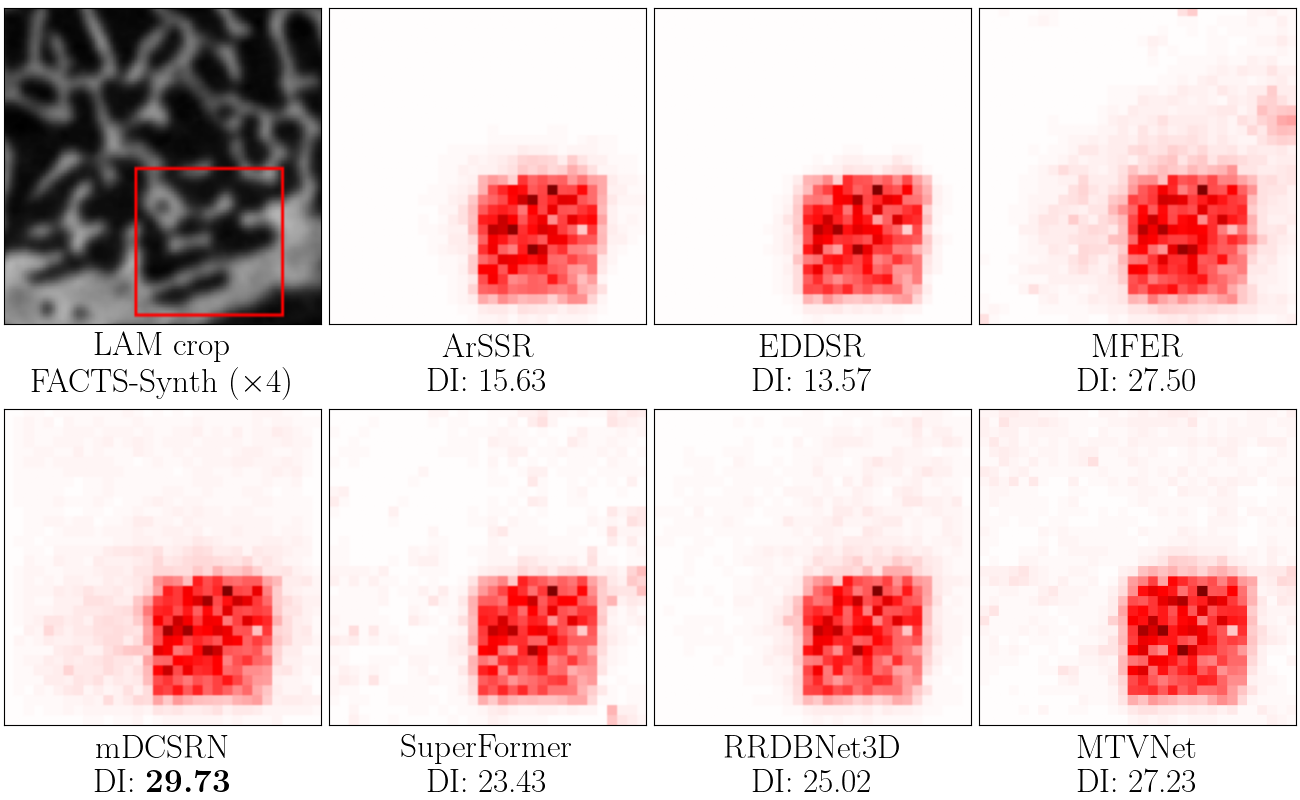}
        %\caption{LAM comparison of SR models from FACTS-Synth at $4 \times$ upscaling.}
        %\label{fig:LAM_visualisation}
        \end{subfigure}
        \caption{LAM comparisons of SR models using FACTS-Synth at $4 \times$ upscaling.}
        \label{fig:LAM_comparisons_supp}
\end{figure}

\section{Visual comparisons using LAM}

The hierarchical architecture of \networkname should ideally help the network take advantage of more surrounding pixels when predicting the SR image. To verify this, we use the LAM attribution method \citep{gu2021interpreting} to analyze the influence of the input pixels on the SR output. The LAM method is a modification of the integrated gradient method \citep{sundararajan2017axiomatic}, specifically designed to investigate SR architectures. It works by accumulating the gradient over interpolations between the input and a blurred version of the input. We have modified the method for 3D analysis and we show the LAM results for all seven model architectures in \cref{fig:LAM_visualisation} for a selected area of a slice and also report the diffusion index (DI), which is a measure of the range of pixels involved in the predicted SR output.

\begin{comment}
\begin{figure*}[h]
  \centering
  \begin{subfigure}{0.49\linewidth}
    \includegraphics[width=1.0\linewidth]{figs/visual_comparisons/SR_comparison_HCP_1200_4x_no_metrics_2_T.png}
    %\caption{Subfigure 1.}
    %\label{fig:subfig1}
  \end{subfigure}
  \hfill
  \begin{subfigure}{0.49\linewidth}
    \includegraphics[width=1.0\linewidth]{figs/visual_comparisons/SR_comparison_IXI_4x_no_metrics_2_T.png}
    %\caption{Subfigure 2.}
    %\label{fig:subfig2}
  \end{subfigure}
  
  \vspace{0.5em} % Space between the rows

  \begin{subfigure}{0.49\linewidth}
    \includegraphics[width=1.0\linewidth]{figs/visual_comparisons/SR_comparison_FACTS_Synth_4x_no_metrics_2_T.png}
    %\caption{Subfigure 3.}
    %\label{fig:subfig3}
  \end{subfigure}
  \hfill
  \begin{subfigure}{0.49\linewidth}
    \includegraphics[width=1.0\linewidth]{figs/visual_comparisons/SR_comparison_FACTS_Real_4x_no_metrics_2_T.png}
    %\caption{Subfigure 4.}
    %\label{fig:subfig4}
  \end{subfigure}
  %\vspace{-0.5em} % Space between the rows
  \caption{Visual comparisons of SR model outputs from the datasets HCP 1200, IXI, FACTS-Synth, and FACTS-Real using $4\times$ upscaling. The ground truth (GT) and LR input images are shown side-by-side in the top-left separated by the red line.}
  \label{fig:visual_comparison}
\end{figure*}
\end{comment}

%\section{Complexity analysis of \networkname}

\section{More visual comparisons}

\begin{figure*}[h]
  \centering
  \begin{subfigure}{0.49\linewidth}
    \includegraphics[width=1.0\linewidth]{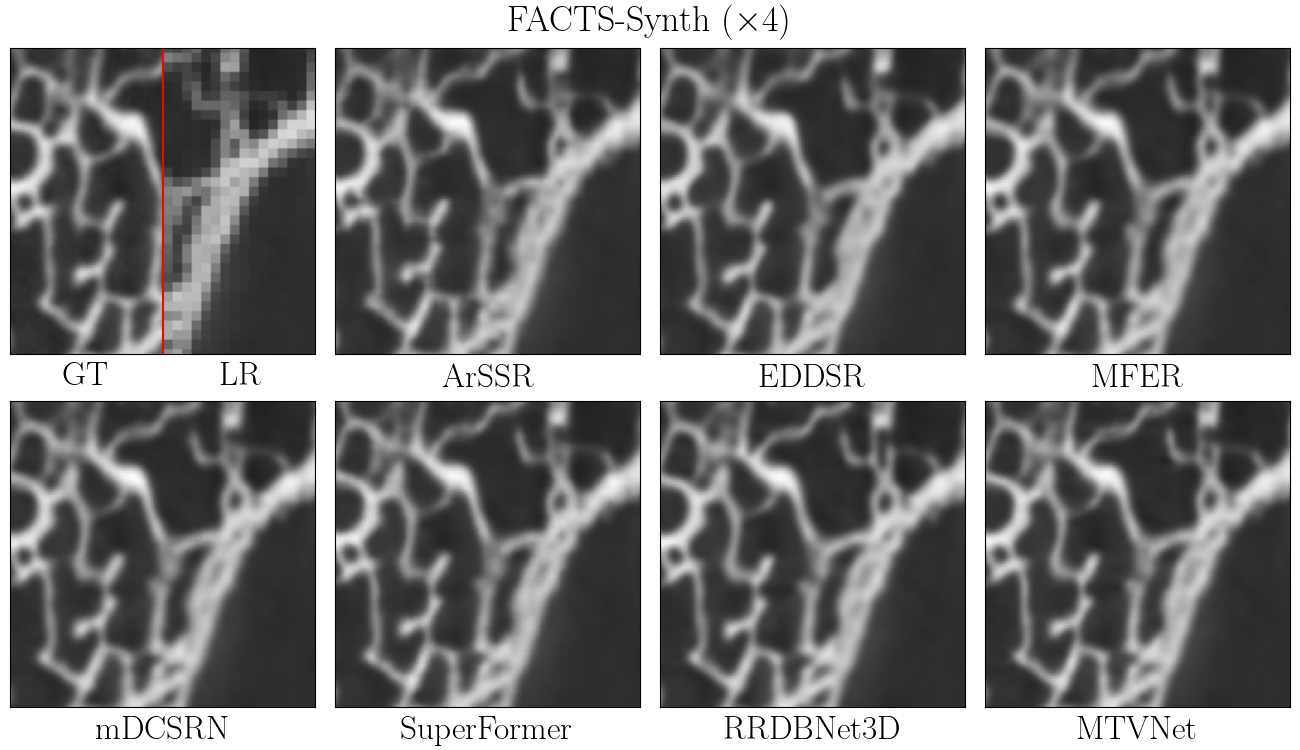}
    %\caption{Subfigure 1.}
    %\label{fig:subfig1}
  \end{subfigure}
  \hfill
  \begin{subfigure}{0.49\linewidth}
    \includegraphics[width=1.0\linewidth]{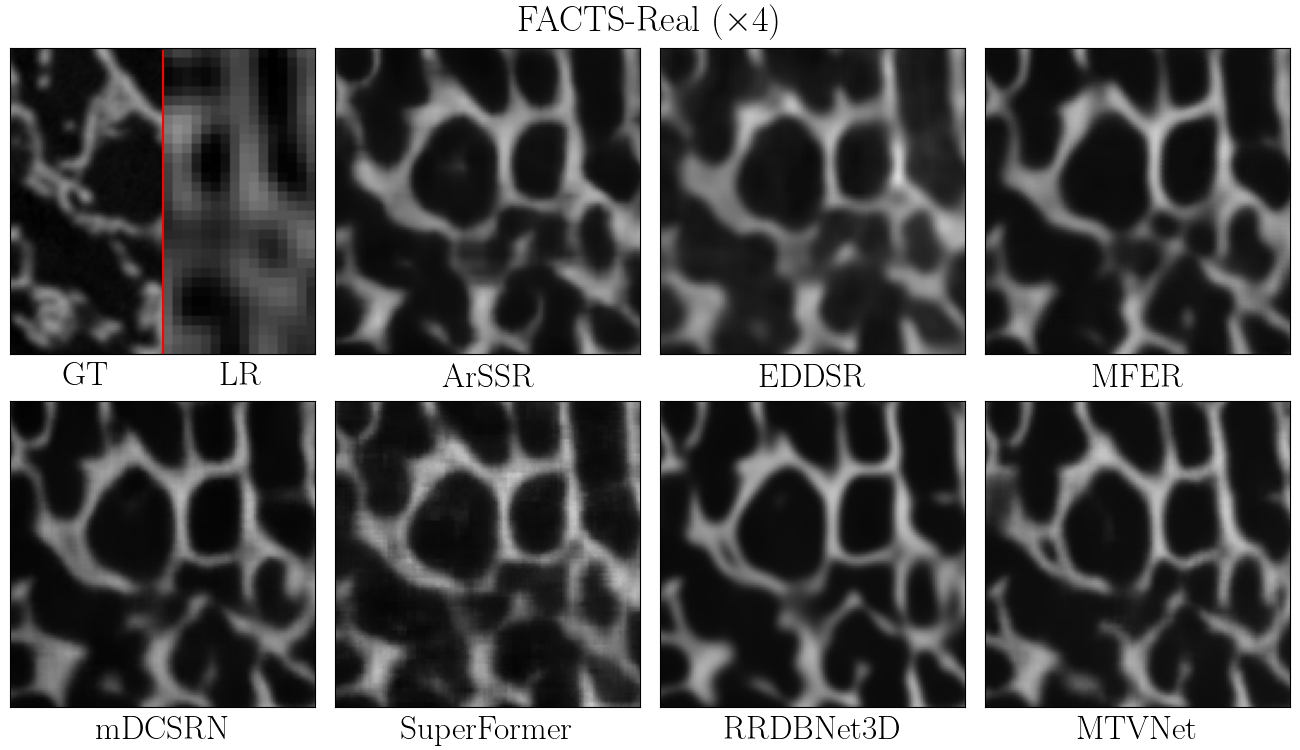}
    %\caption{Subfigure 2.}
    %\label{fig:subfig2}
  \end{subfigure}
  
  \vspace{0.5em} % Space between the rows

  \begin{subfigure}{0.49\linewidth}
    \includegraphics[width=1.0\linewidth]{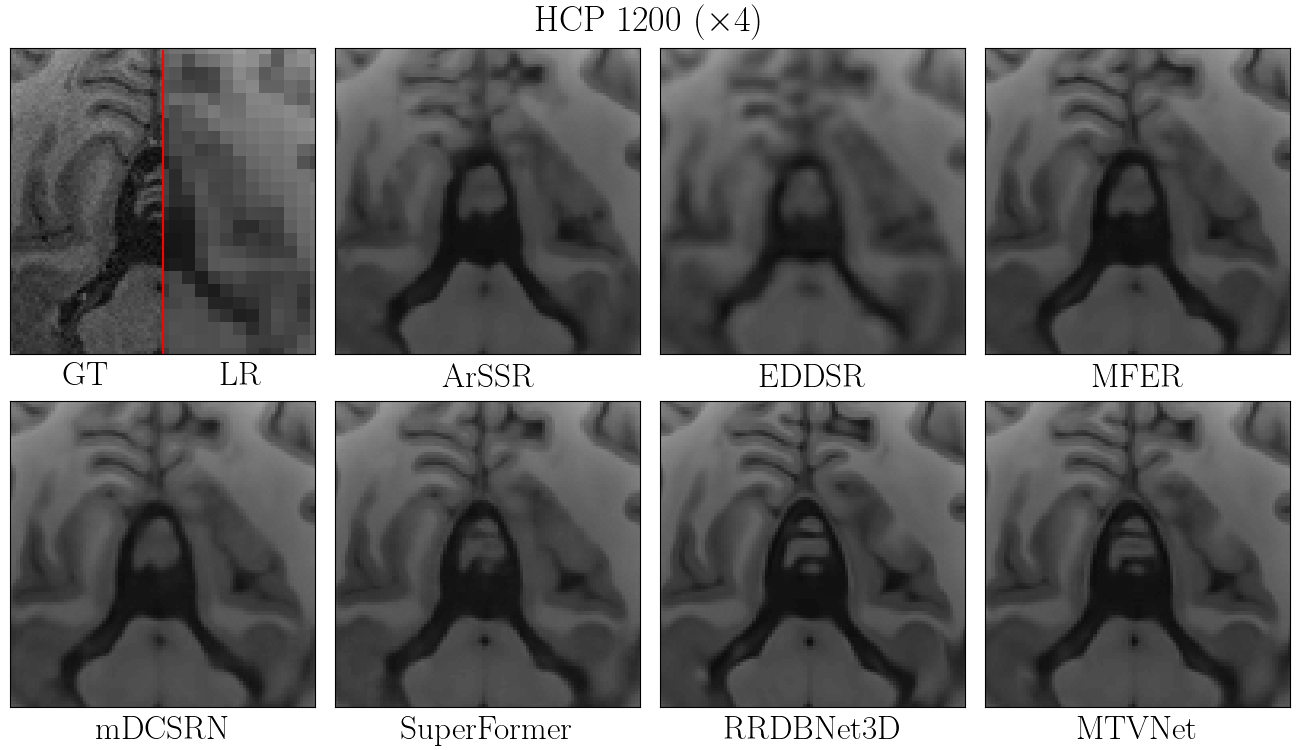}
    %\caption{Subfigure 3.}
    %\label{fig:subfig3}
  \end{subfigure}
  \hfill
  \begin{subfigure}{0.49\linewidth}
    \includegraphics[width=1.0\linewidth]{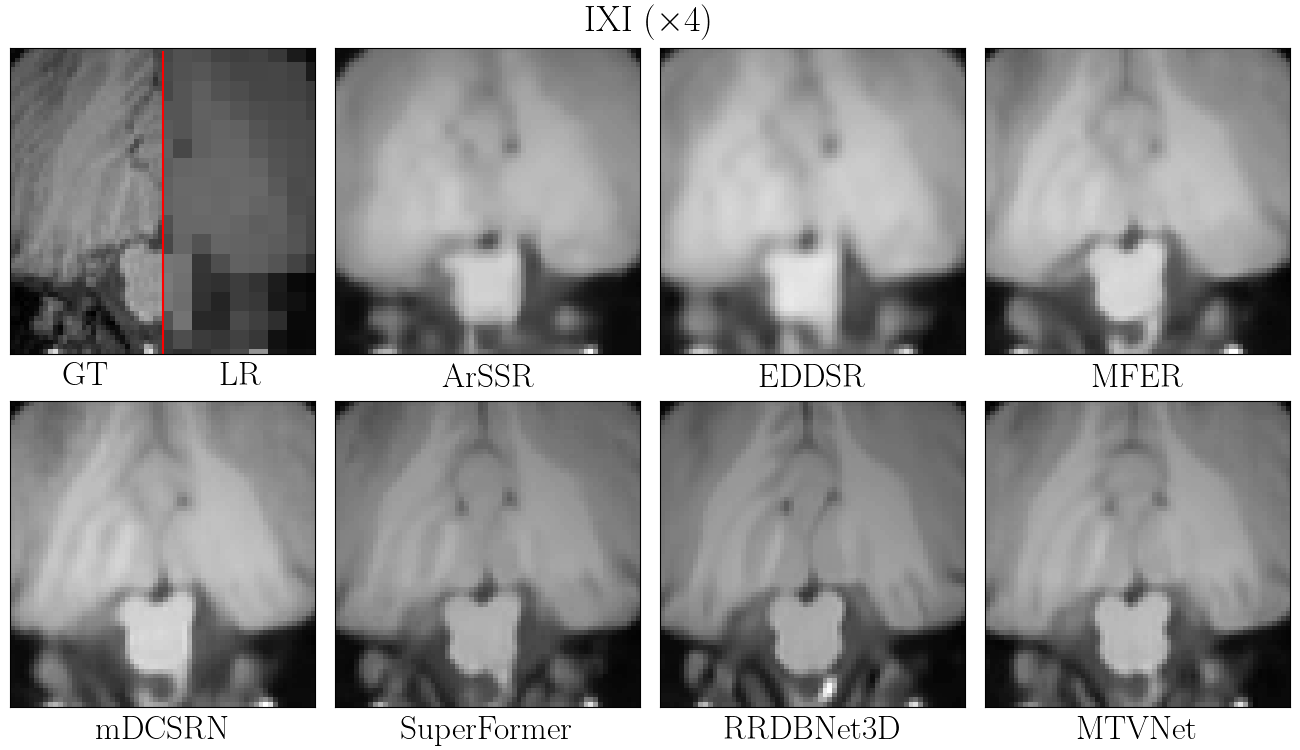}
    %\caption{Subfigure 4.}
    %\label{fig:subfig4}
  \end{subfigure}

  \vspace{0.5em} % Space between the rows

  \begin{subfigure}{0.49\linewidth}
    \includegraphics[width=1.0\linewidth]{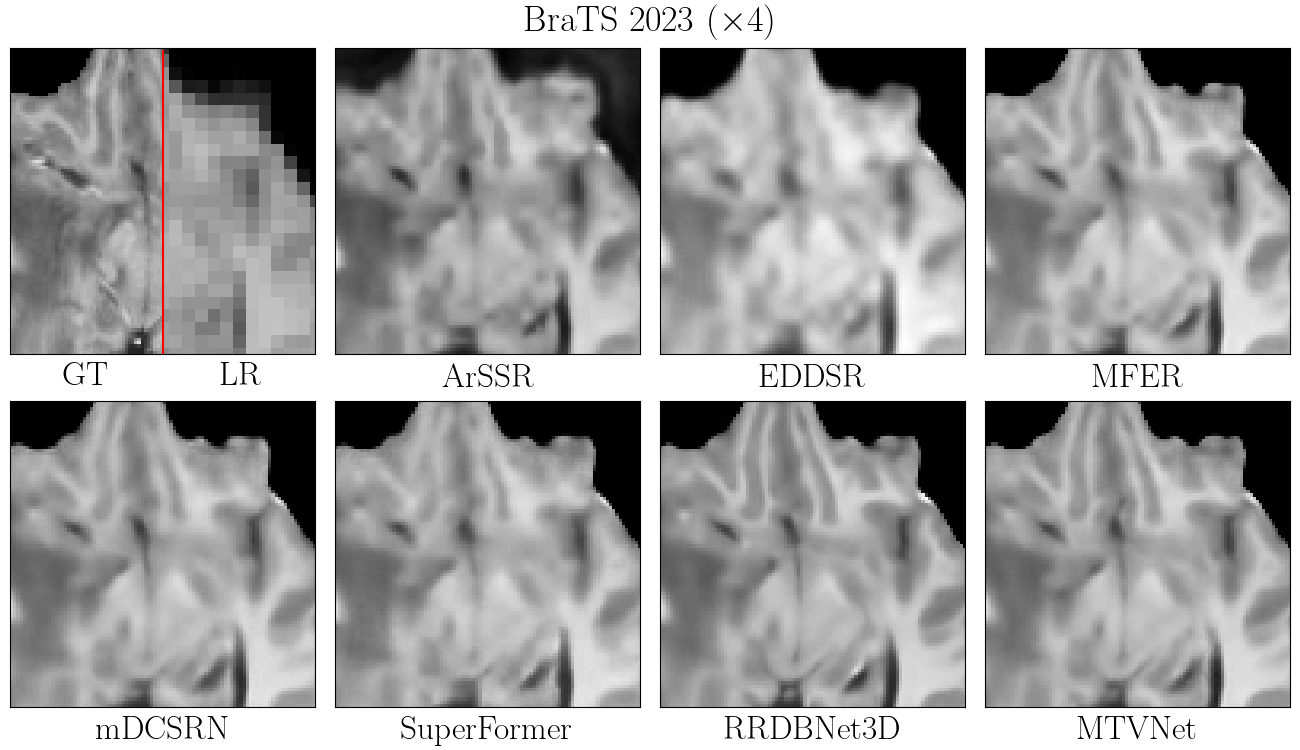}
    %\caption{Subfigure 3.}
    %\label{fig:subfig3}
  \end{subfigure}
  \hfill
  \begin{subfigure}{0.49\linewidth}
    \includegraphics[width=1.0\linewidth]{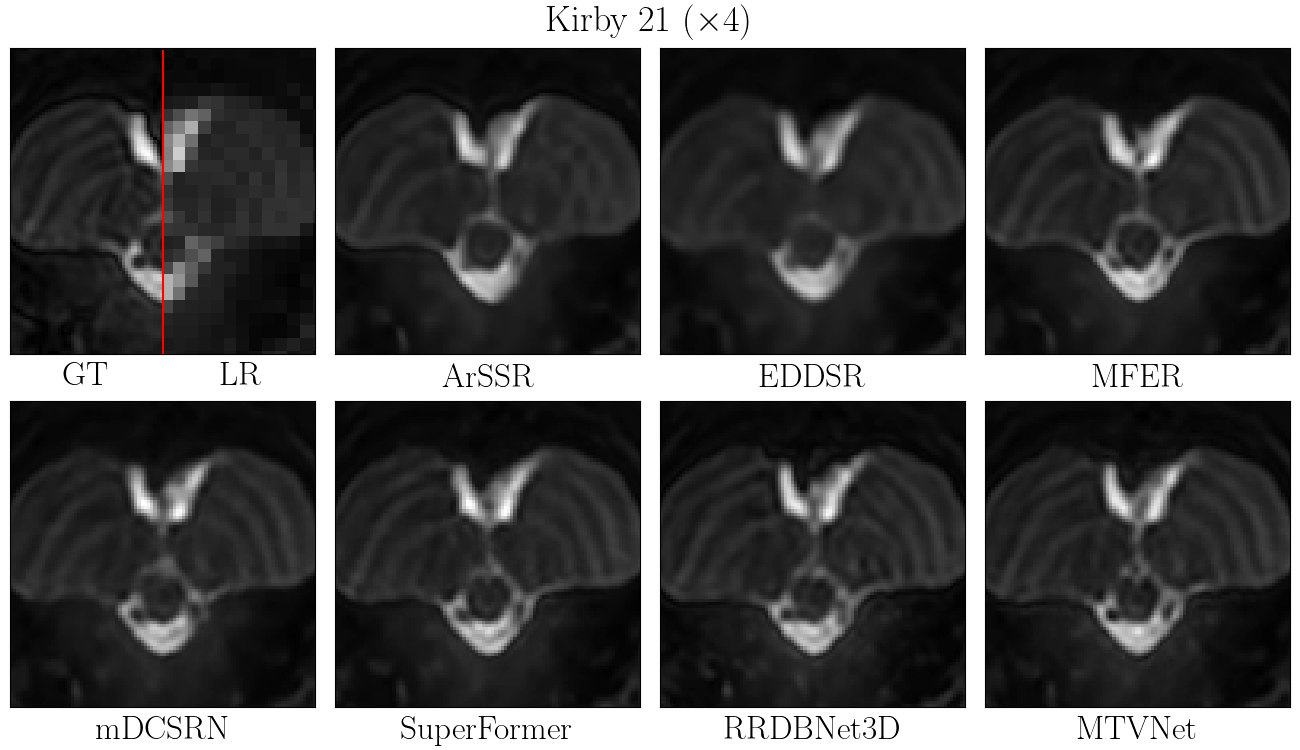}
    %\caption{Subfigure 4.}
    %\label{fig:subfig4}
  \end{subfigure}
  %\vspace{-0.5em} % Space between the rows
  \caption{Visual comparisons of SR model outputs from the datasets HCP 1200, IXI, FACTS-Synth, and FACTS-Real using $4\times$ upscaling. The ground truth (GT) and LR input images are shown side-by-side in the top-left separated by the red line.}
  \label{fig:visual_comparison}
\end{figure*}

\iffalse
\section{Rationale}
\label{sec:rationale}
% 
Having the supplementary compiled together with the main paper means that:
% 
\begin{itemize}
\item The supplementary can back-reference sections of the main paper, for example, we can refer to \cref{sec:intro};
\item The main paper can forward reference sub-sections within the supplementary explicitly (e.g. referring to a particular experiment); 
\item When submitted to arXiv, the supplementary will already included at the end of the paper.
\end{itemize}
% 
To split the supplementary pages from the main paper, you can use \href{https://support.apple.com/en-ca/guide/preview/prvw11793/mac#:~:text=Delete%20a%20page%20from%20a,or%20choose%20Edit%20%3E%20Delete).}{Preview (on macOS)}, \href{https://www.adobe.com/acrobat/how-to/delete-pages-from-pdf.html#:~:text=Choose%20%E2%80%9CTools%E2%80%9D%20%3E%20%E2%80%9COrganize,or%20pages%20from%20the%20file.}{Adobe Acrobat} (on all OSs), as well as \href{https://superuser.com/questions/517986/is-it-possible-to-delete-some-pages-of-a-pdf-document}{command line tools}.
\fi
